# Supplementary material for: One Explanation is Not Enough: Structured Attention Graphs for Image Classification
Source: arXiv:2011.06733 source file (2021-11-07)
Supplement: Supplementary file 1 [file appendixB.tex]

A flowchart illustrating the steps involved to generate a SAG for a given image input.

%%%%%%%%%%%%%%%%%%%%
\begin{figure}[!h]
    \centering
    \includegraphics[width = \textwidth]{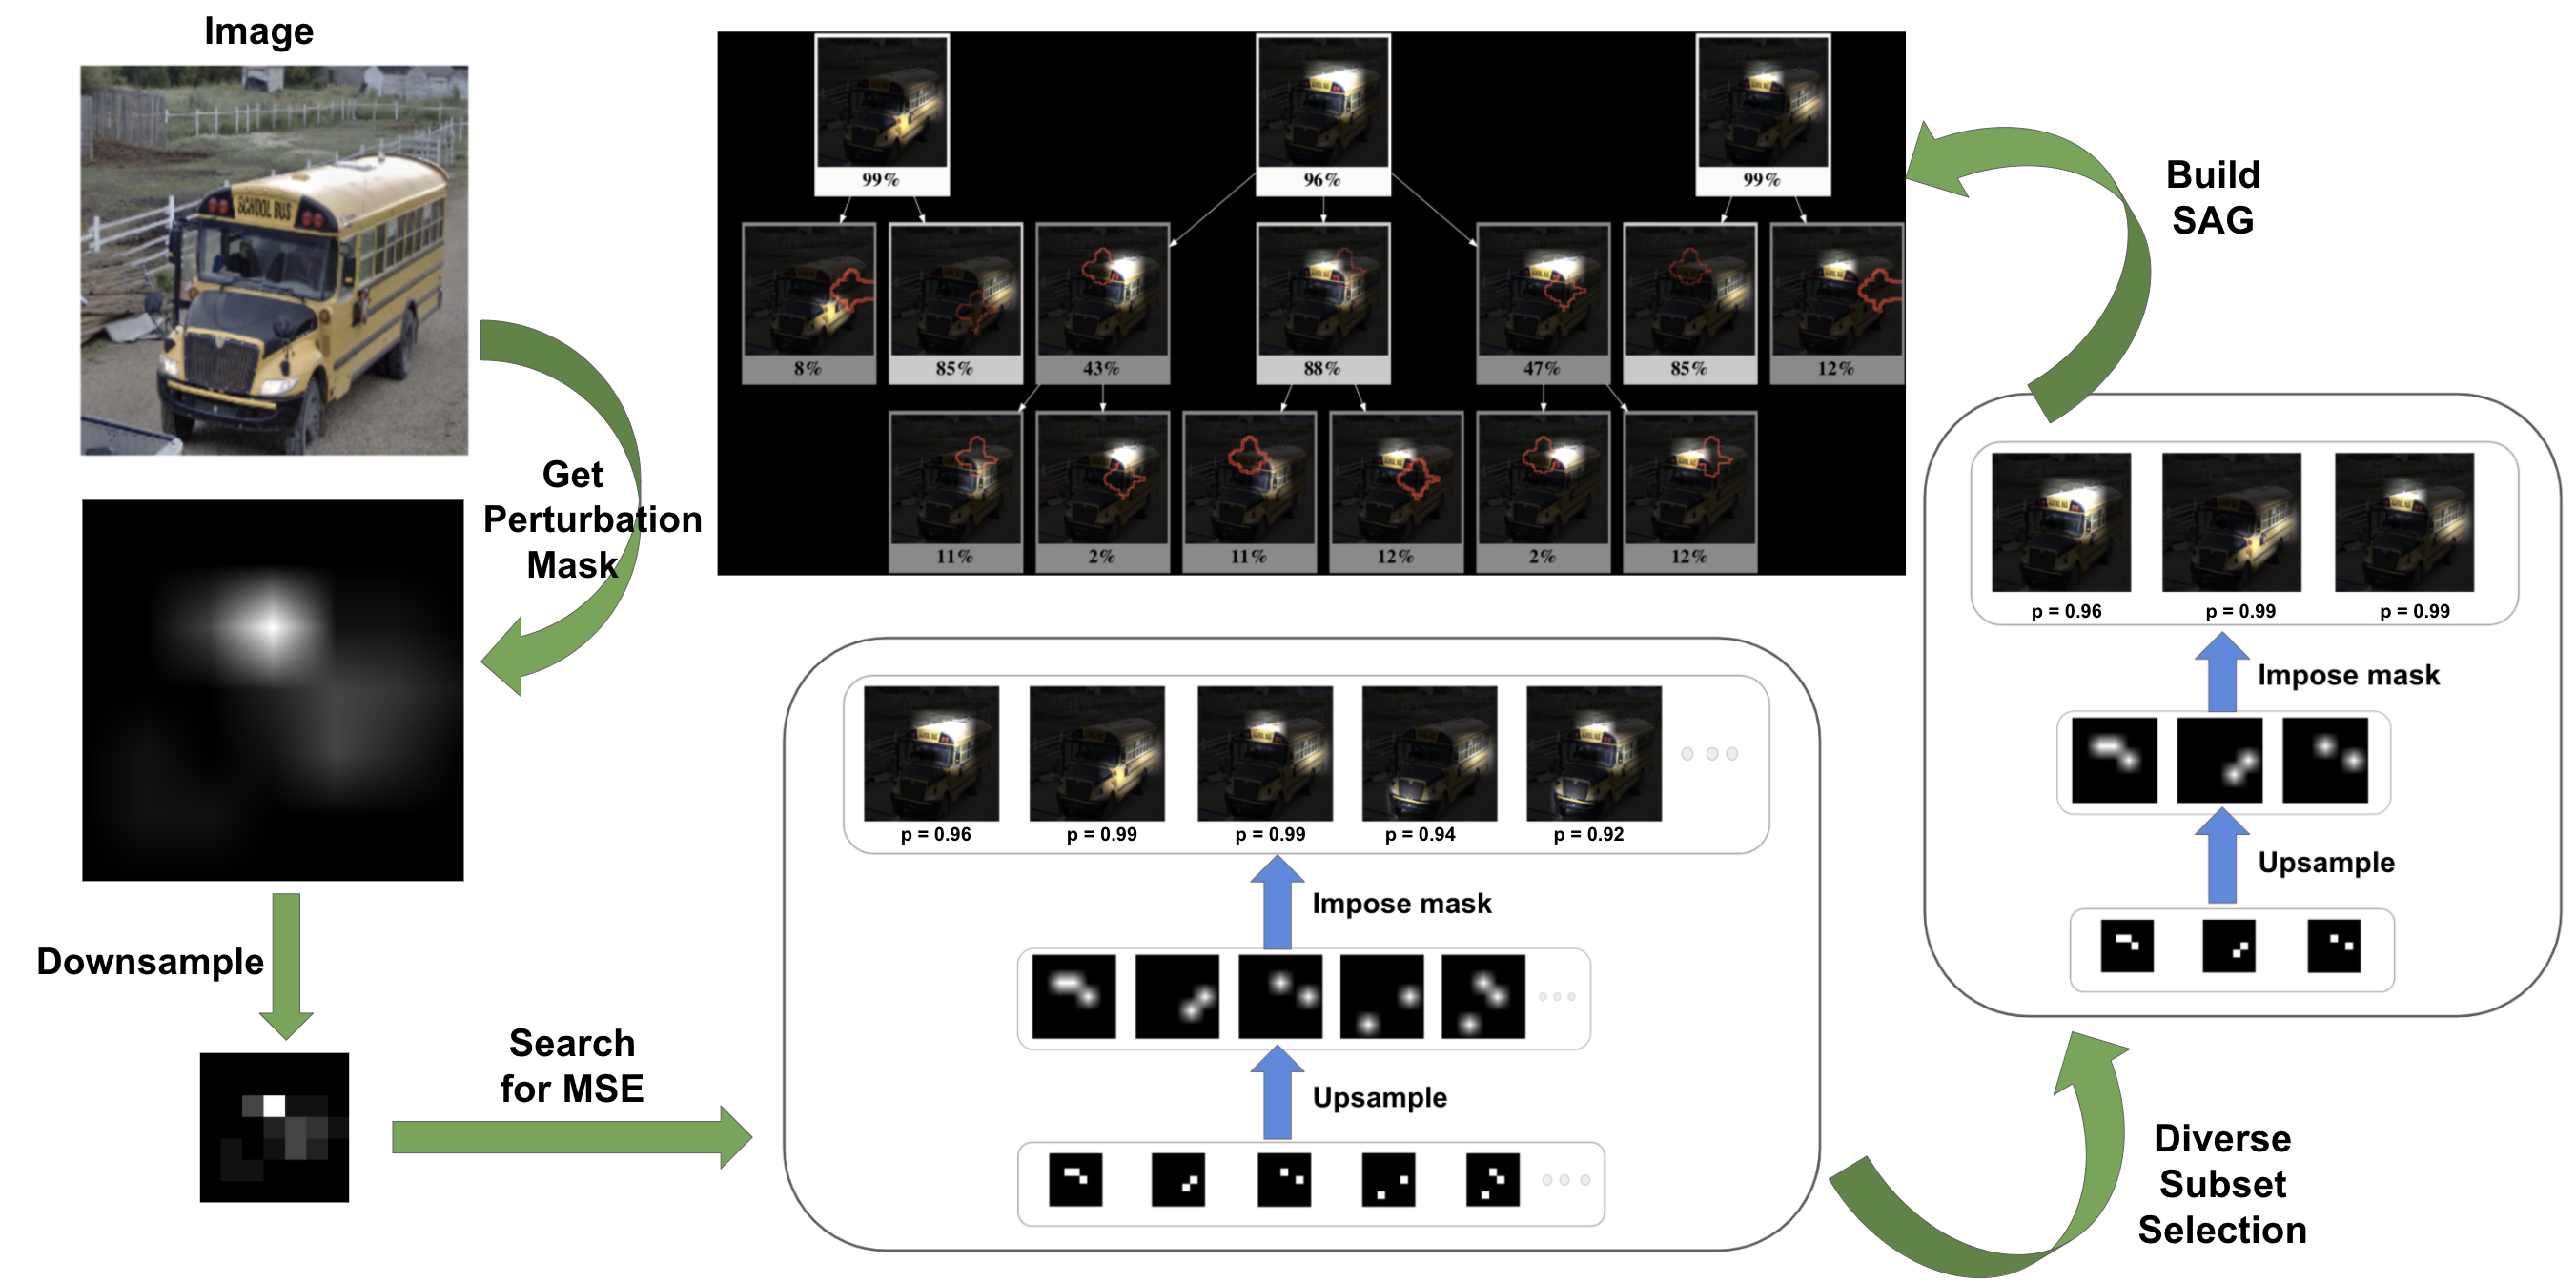}
    %\vspace{-5pt}
    \caption{Illustration of the steps for generating a SAG (on top middle) from a given image (on top left).
    }
    \label{fig:method_summary}
\end{figure}
%%%%%%%%%%%%%%%%%%%%
